# Supplementary material for: RobustFill: Neural Program Learning under Noisy I/O
Source: arXiv:1703.07469 source file (2017-03-21)
Supplement: Supplementary file 1 [file supplementary.tex]

% This figure is from the removed section: Generalization beyond the DSL


% \subsection{Generalizing Beyond the DSL}

% It is obvious that a synthesis model cannot generalize beyond the DSL it was trained on, but it is less clear to what extend an induction model is able to do this.\footnote{The term ``generalize'' is being overloaded somewhat here. In this case it means generalizing from training to test, while previously it meant generalizing from observed examples to held-out examples.} To test this, we created two augmented versions of the FlashfillTest set. No changes were made to the trained model or decoder. The two augmentations are:

% \begin{itemize}
% \item {\bf Concat}: One powerful way of selecting substrings using the DSL is the $GetToken()$ and $GetSpan()$ functions, which take a token index (not character) as a parameter. These were trained up to index 5.\footnote{This is an arbitrary hyperparameter that can be changed during data synthesis.} For this augmentation, we concatenate strings from three random test instances to create much longer IO examples. The goal is to create instances with longer token sequences than the models were trained on, so the synthesis model is not able to emit the appropriate position tokens.
% \item {\bf Delim}: Several important DSL functions, including $GetToken()$ and $GetSpan()$, make use of Unicode character classes to split the character string into tokens. For example, if $I = $ {\tt john,mary,sue} and $P =$ \t{GetToken(Word, 2)}, then $O = $ {\tt mary}. Here, we replace all delimiter tokens in both $I$ and $O$ with rare letter tokens: period $\rightarrow$ 'z', space $\rightarrow$ 'q', comma $\rightarrow$ 'x', and so on. The test instances will still generally be solvable (by {\it some} DSL), but the synthesis model cannot emit delimiter-based tokenization functions.
% \end{itemize}

% Note that the augmentations were applied to both observed and held-out examples, and the two augmentation types were applied separately.

% Results are shown in Figure~\ref{fig:data_aug_results}. On the ``Concat'' augmentation, induction has a greater degradation in performance than synthesis w/ beam=100, but a smaller degradation than synthesis w/ beam=1. On the ``Delim'' augmentation, induction has a greater degradation in performance than both synthesis models.

% Therefore, these results provide some evidence against the hypothesis that induction models have an {\it intrinsic} strength at generalizing beyond the DSL they were trained on. Of course, it must be noted that these augmentations were not created rigorously with respect to an expanded DSL, and they also introduce other confounding factors such as the length of the input string. A more formal study is need to draw more certain conclusions.

% \begin{figure}
% \begin{center}
% \begin{tabular}{|l|c|c|c|}
% \hline
% & \multicolumn{3}{|c|}{\textbf{Avg-Example Accuracy}} \\ \hline
% & \textbf{Base} & \textbf{Concat} & \textbf{Delim} \\ \hline
% Synthesis, Beam=1 & 54\% & 16\% & 30\% \\ \hline
% Synthesis, Beam=100 & 84\% & 53\% & 59\% \\ \hline
% Induction & 73\% & 37\% & 45\% \\ \hline
% \end{tabular}
% \end{center}
% \caption{Average-example accuracy on augmented versions of FlashfillTest.}
% \label{fig:data_aug_results} 
% \end{figure}


% \subsection{Search Space of Program Synthesis}
% \label{sec:search_space}

% The search space of a non-statistical synthesis algorithm is dependent on the amount of effort put into manually specifying the inverse function semantics and search pruning rules. Previous work in non-statistical modeling of Flashfill \cite{gulwani2012,gulwani2011} involves a large amount of work in hand-coding the inverse function semantics. It also uses a DSL with a much smaller set of unique expressions. Significant effort would be required to extend that method to the DSL described here, and to more complicated future DSLs.

% A more general approach to analyzing the search space of our DSL is to only consider ``black-box'' synthesis algorithms which do not encode specific inverse function semantics. A naive search will clearly be exponential with respect to the maximum program length, but this can be substantially improved upon by taking advantage of the concatenative nature of our DSL. After each candidate expression is generated, it can be executed using the DSL, and if the resulting string is inconsistent with $O_j$, that expression can be discarded. This search can be efficiently performed using dynamic programming, where a lattice of solutions is constructed based on character positions within each $O_j$. However, it is important to note that such black-box pruning can only be performed on {\it complete} expressions. 

% For a single IO example, this algorithm has a cost of $O(c*e)$, where $c$ is the maximum number characters in each $O_j$, and $e$ is the maximum number of unique expressions. In our experiments, $c = 100$, and $e$ can be computed from our DSL specification.

% In terms of search space, the dominating function in our DSL is \t{GetSpan()}. This function has 6 parameters, which have 26 * 10 * 2 * 26 * 10 * 2 = 270,400 possible expansions. This function can be nested as the child of approximately 100 other sub-expressions, resulting in 27,040,000 unique expressions containing just \t{GetSpan()}. Note that this function is critical to the DSL -- roughly 20\% of the instances in FlashfillTest cannot be solved when it is removed. The remaining functions can be expanded to roughly 3 million unique expressions, resulting in $e = 30,000,000$ total unique expressions. The total search cost is thus on the order of $100*30,000,000 \approx 10^9$ program evaluations, which is bordering intractable for most real-world applications.

% Additionally, this analysis is only for a single, non-noisy IO-example -- the search cost increases significantly when operating on multiple IO examples, and the algorithm fails completely when any noise is introduced to either the {\tt InStr} or {\tt OutStr}. The performance of \citet{gulwani2012} on noisy IO is detailed in Section~\ref{sec:noise}.

% \section{DSL Semantics}
